# Supplementary material for: Thermoelectric transport trends in group 4 half-Heusler alloys
Source: arXiv:1907.02845 source file (2019-07-05)
Supplement: Supplementary file 1 [file Supplementary.pdf]

# Thermoelectric transport trends in group 4 half-Heusler alloys — Supplmenetary material

Kristian Berland,[1,2,*] Nina Shulumba,[3] Olle Hellman,[3] Clas Persson,[2] and Ole Martin Løvvik[2,4]

[1] *Faculty of Science and Technology, Norwegian University of Life Sciences, Norway.*
[2] *Centre for Materials Science and Nanotechnology, Department of Physics, University of Oslo, Norway*
[3] *Department of Applied Physics & Materials Science, California Institute of Technology, Pasadena, CA, United States*
[4] *SINTEF Materials Physics, NO–0314 Oslo, Norway*

## I. THERMAL CONDUCTIVITY

| | $\overline{\nu}$ [km/s] | $\kappa_\ell$ [W/Km] | $\kappa_\ell^{\mathrm{md-x}}$ [W/Km] | $\kappa_\ell^{\mathrm{md-z}}$ [W/Km] | $\kappa_\ell^{\mathrm{md-x,gb}}$ [W/Km] | $\kappa_\ell^{\mathrm{md-x,gb}}$ [W/Km] |
|---|---|---|---|---|---|---|
| *stable* | | | | | | |
| TiNiSn | 3.97 | 6.18 | 2.48 | 2.65 | **1.77** | 1.86 |
| TiPdSn | 3.44 | 4.01 | 2.25 | 2.33 | 1.57 | **1.53** |
| TiPtSn | 3.31 | 6.48 | 3.95 | 4.02 | 2.52 | **2.27** |
| ZrNiSn | 3.83 | 6.58 | 3.34 | 3.06 | 2.44 | **2.22** |
| ZrPdSn | 3.50 | 5.93 | 3.33 | 2.90 | 2.25 | **1.84** |
| ZrPtSn | 3.32 | 6.17 | 4.21 | 3.40 | 2.94 | **2.17** |
| ZrNiPb | 3.22 | 5.60 | 3.75 | 1.92 | 2.69 | **1.32** |
| ZrPdPb | 2.97 | 3.87 | 2.96 | 1.96 | 1.96 | **1.21** |
| ZrPtPb | 2.85 | 3.74 | 3.08 | 2.14 | 2.04 | **1.36** |
| HfNiSn | 3.35 | 6.70 | 2.63 | 4.15 | **1.83** | 2.82 |
| HfPdSn | 3.11 | 5.75 | 3.11 | 3.42 | **2.03** | 2.27 |
| HfPtSn | 3.02 | 6.54 | 4.15 | 3.73 | 2.83 | **2.45** |
| HfNiPb | 2.89 | 6.48 | 2.95 | 2.35 | 2.06 | **1.68** |
| HfPdPb | 2.66 | 3.57 | 3.00 | 2.24 | 1.85 | **1.54** |
| HfPtPb | 2.61 | 3.35 | 3.42 | 2.55 | 2.28 | **1.71** |
| TiCoSb | 4.07 | 8.39 | 2.73 | 3.19 | **2.02** | 2.35 |
| TiRhSb | 3.67 | 6.72 | 3.11 | 2.92 | 2.17 | **1.85** |
| TiIrAs | 3.60 | 9.08 | 4.97 | 3.85 | 3.46 | **2.45** |
| TiIrSb | 3.41 | 6.78 | 4.04 | 3.86 | 2.87 | **2.52** |
| ZrCoSb | 3.96 | 8.49 | 3.62 | 3.29 | 2.86 | **2.58** |
| ZrRhSb | 3.69 | 7.10 | 3.32 | 2.99 | 2.40 | **2.08** |
| ZrCoBi | 3.32 | 6.82 | 3.97 | 2.10 | 3.03 | **1.60** |
| ZrRhBi | 3.12 | 4.59 | 3.15 | 1.91 | 2.30 | **1.26** |
| ZrIrAs | 3.41 | 4.59 | 3.16 | 3.21 | 2.35 | **2.34** |
| ZrIrSb | 3.47 | 6.77 | 4.36 | 3.42 | 3.25 | **2.37** |
| ZrIrBi | 2.96 | 4.52 | 3.54 | 2.60 | 2.47 | **1.69** |
| HfCoSb | 3.47 | 8.32 | 2.79 | 4.60 | **2.08** | 3.35 |
| HfRhSb | 3.27 | 7.00 | 3.34 | 3.83 | **2.23** | 2.56 |
| HfRhBi | 2.75 | 4.44 | 3.27 | 2.39 | 2.25 | **1.70** |
| HfIrSb | 3.14 | 8.46 | 4.71 | 4.31 | 3.29 | **3.08** |
| *unstable* | | | | | | |
| TiNiPb | 2.84 | 8.65 | 2.54 | 1.34 | 2.01 | **0.91** |
| TiPdPb | 2.47 | 3.80 | 2.47 | 1.64 | **1.60** | 0.99 |
| TiPtPb | 2.70 | 3.67 | 2.50 | 1.82 | 1.62 | **1.15** |
| TiCoBi | 2.87 | 6.59 | 2.74 | 1.46 | 2.27 | **1.12** |
| TiRhBi | 2.48 | 2.16 | 1.57 | 1.06 | 1.23 | **0.78** |
| HfCoBi | 2.95 | 7.55 | 3.18 | 2.60 | 2.49 | **2.00** |
| HfIrBi | 2.72 | 4.39 | 3.81 | 2.89 | 2.61 | **1.97** |
| TiNiGe | 4.57 | 9.20 | 2.58 | 2.56 | 1.70 | **1.57** |
| TiPdGe | 3.81 | 7.51 | 3.19 | 2.55 | 2.08 | **1.44** |
| TiPtGe | 3.52 | 8.54 | 4.53 | 3.60 | 2.89 | **2.14** |
| ZrNiGe | 4.14 | 7.27 | 2.95 | 2.35 | 2.05 | **1.64** |
| ZrPdGe | 3.64 | 6.36 | 3.24 | 2.76 | 2.05 | **1.72** |
| ZrPtGe | 3.32 | 5.05 | 3.42 | 3.27 | 2.35 | **2.21** |
| HfNiGe | 3.54 | 7.09 | 2.43 | 3.88 | **1.59** | 2.34 |
| HfPdGe | 3.19 | 6.15 | 2.93 | 3.85 | **1.83** | 2.48 |
| HfPtGe | 3.04 | 7.10 | 4.00 | 4.30 | **2.54** | 2.82 |
| TiCoAs | 4.70 | 12.29 | 2.47 | 2.51 | 1.73 | **1.70** |
| TiRhAs | 4.00 | 10.89 | 4.05 | 2.70 | 2.72 | **1.57** |
| ZrCoAs | 4.22 | 8.40 | 2.89 | 2.12 | 2.31 | **1.60** |
| ZrRhAs | 3.82 | 8.30 | 3.26 | 2.78 | 2.26 | **1.85** |
| HfCoAs | 3.63 | 6.94 | 2.35 | 3.07 | **1.73** | 2.26 |
| HfRhAs | 3.32 | 6.79 | 3.16 | 3.79 | **2.08** | 2.60 |
| HfIrAs | 3.08 | 5.54 | 3.63 | 3.48 | **2.50** | 2.63 |

TABLE S1. Average accoustic phonon velocity $\overline{\nu} = (\nu_l + 2\nu_t)/3$ and thermal conductivity for all compounds studies, $\kappa_\ell$ includes only intrinsic scattering mechanisms, $\kappa_\ell^{\mathrm{md-x(md-z)}}$ includes mass-disorder scattering on the X (Z) site as described in the text, whereas $\kappa_\ell^{\mathrm{md-x(md-z),gb}}$ also includes grain-boundary scattering, where the boldface indidcates the smallest of the two values and is used in the estimate of $ZT$.

### A. Thermal conductivity at $T = 300\text{K}$

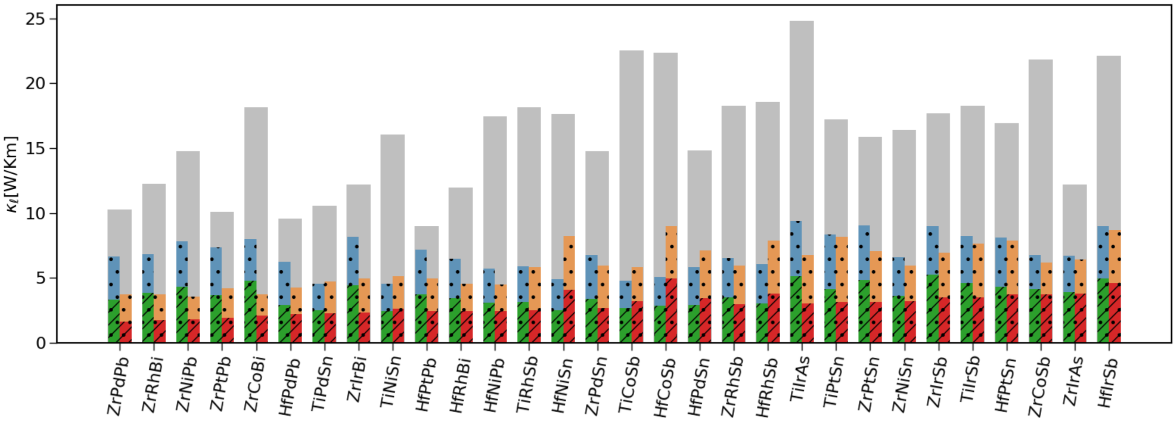


FIG. S1. The phonon thermal conductivity $\kappa_\ell$ at $T = 300$ K due to anharmonic phonon-phonon scattering (grey bars), with alloy scattering included on the $X$ site (blue) and the $Z$ site (yellow), and with grain boundary scattering combined with alloy scattering on the $X$ site (green) and the $Z$ site (red). Alloy scattering (dotted bars) was achieved with 12.5% isoelectronic substitution in the VCA, as explained in the text. Grain boundary scattering (striped bars) assumed a typical grain size of 100 nm. The compounds are listed from left to right according to the lowest calculated $\kappa_\ell$ achieved with any combination of scattering mechanisms.

### B. Thermal conductivity as function of grain size

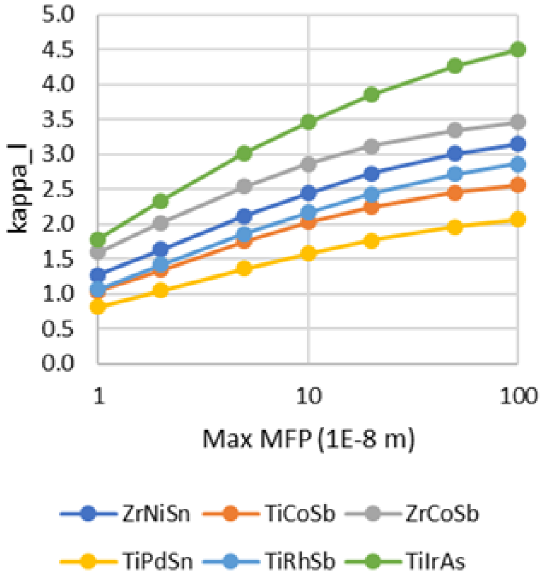


FIG. S2. Effect of grain boundary size on thermal conducitiy og the six selected compounds at 800 K.

## II. THERMOELECTRIC PROPERTIES

### A. Results with hybrid functional HSE and $\tau = 10^{-14}$s

| | $\kappa_\ell^{\min}$ [W/Km] | n [$10^{20}$/cm$^3$] | $\kappa_e$ [W/Km] | $\sigma$ [$10^4$S/m] | $S$ [$\mu$W/K] | $\mathcal{P}$[mW/K$^2$m] | $ZT$ |
|---|---|---|---|---|---|---|---|
| *stable* | | | | | | | |
| TiNiSn | 1.77 | 1.01 | 0.99 | 6.28 | -242 | 3.69 | 1.07 |
| TiPdSn | 1.53 | 1.36 | 0.86 | 5.53 | -255 | 3.59 | 1.20 |
| TiPtSn | 2.27 | 3.13 | 1.41 | 8.31 | -253 | 5.33 | 1.16 |
| ZrNiSn | 2.22 | 0.93 | 1.07 | 6.90 | -234 | 3.79 | 0.92 |
| ZrPdSn | 1.84 | 0.97 | 0.92 | 6.04 | -244 | 3.58 | 1.04 |
| ZrPtSn | 2.17 | 1.63 | 1.03 | 6.65 | -238 | 3.76 | 0.94 |
| ZrNiPb | 1.32 | 0.90 | 1.15 | 6.68 | -234 | 3.66 | 1.18 |
| ZrPdPb | 1.21 | 0.86 | 0.84 | 5.32 | -255 | 3.46 | 1.35 |
| ZrPtPb | 1.36 | 1.28 | 0.78 | 5.13 | -260 | 3.47 | 1.29 |
| HfNiSn | 1.83 | 0.98 | 1.17 | 7.11 | -232 | 3.83 | 1.02 |
| HfPdSn | 2.03 | 1.06 | 1.00 | 6.50 | -239 | 3.73 | 0.98 |
| HfPtSn | 2.45 | 1.73 | 1.09 | 7.05 | -233 | 3.84 | 0.87 |
| HfNiPb | 1.68 | 1.26 | 1.85 | 9.88 | -200 | 3.96 | 0.90 |
| HfPdPb | 1.54 | 0.99 | 1.06 | 6.47 | -240 | 3.73 | 1.15 |
| HfPtPb | 1.71 | 1.36 | 0.91 | 5.85 | -250 | 3.65 | 1.12 |
| TiCoSb | 2.02 | 3.45 | 1.10 | 7.41 | -255 | 4.82 | 1.23 |
| TiRhSb | 1.85 | 6.34 | 1.25 | 9.31 | -276 | 7.09 | 1.83 |
| TiIrAs | 2.45 | 6.38 | 3.05 | 19.34 | -242 | 11.29 | 1.64 |
| TiIrSb | 2.52 | 5.87 | 1.88 | 12.43 | -247 | 7.56 | 1.37 |
| ZrCoSb | 2.58 | 3.26 | 1.38 | 9.20 | -253 | 5.87 | 1.19 |
| ZrRhSb | 2.08 | 3.13 | 1.24 | 7.97 | -264 | 5.56 | 1.34 |
| ZrCoBi | 1.60 | 2.18 | 1.02 | 6.80 | -273 | 5.06 | 1.55 |
| ZrRhBi | 1.26 | 2.15 | 0.92 | 6.36 | -292 | 5.41 | 1.99 |
| ZrIrAs | 2.34 | 42.43 | 25.38 | 134.82 | -75 | 7.50 | 0.22 |
| ZrIrSb | 2.37 | 6.42 | 2.39 | 14.25 | -252 | 9.05 | 1.52 |
| ZrIrBi | 1.69 | 34.72 | 17.19 | 91.79 | -90 | 7.50 | 0.32 |
| HfCoSb | 2.08 | 2.63 | 1.22 | 8.14 | -263 | 5.63 | 1.36 |
| HfRhSb | 2.23 | 2.98 | 1.29 | 8.56 | -261 | 5.84 | 1.32 |
| HfRhBi | 1.70 | 5.83 | 5.40 | 26.43 | -152 | 6.10 | 0.69 |
| HfIrSb | 3.08 | 16.57 | 8.44 | 42.32 | -149 | 9.37 | 0.65 |
| *unstable* | | | | | | | |
| TiNiPb | 0.91 | 1.26 | 1.08 | 6.17 | -240 | 3.54 | 1.42 |
| TiPdPb | 0.99 | 1.40 | 0.72 | 4.72 | -264 | 3.28 | 1.54 |
| TiPtPb | 1.15 | 2.54 | 0.68 | 4.91 | -265 | 3.46 | 1.51 |
| TiCoBi | 1.12 | 2.20 | 0.75 | 5.14 | -280 | 4.03 | 1.72 |
| TiRhBi | 0.78 | 3.96 | 0.66 | 4.73 | -308 | 4.47 | 2.49 |
| HfCoBi | 2.00 | 2.26 | 1.19 | 7.87 | -264 | 5.49 | 1.38 |
| HfIrBi | 1.97 | 0.30 | 0.83 | 4.15 | -100 | 0.41 | 0.12 |
| TiNiGe | 1.57 | 1.32 | 0.87 | 5.83 | -257 | 3.85 | 1.26 |
| TiPdGe | 1.44 | 1.84 | 0.83 | 5.48 | -263 | 3.78 | 1.33 |
| TiPtGe | 2.14 | 4.74 | 1.36 | 9.31 | -265 | 6.55 | 1.50 |
| ZrNiGe | 1.64 | 0.99 | 0.91 | 6.11 | -259 | 4.08 | 1.28 |
| ZrPdGe | 1.72 | 1.21 | 0.93 | 6.25 | -256 | 4.08 | 1.23 |
| ZrPtGe | 2.21 | 2.25 | 1.13 | 7.32 | -246 | 4.42 | 1.06 |
| HfNiGe | 1.59 | 0.96 | 0.91 | 6.12 | -260 | 4.13 | 1.32 |
| HfPdGe | 1.83 | 1.22 | 0.99 | 6.59 | -255 | 4.28 | 1.22 |
| HfPtGe | 2.54 | 2.32 | 1.26 | 8.00 | -242 | 4.69 | 0.99 |
| TiCoAs | 1.70 | 3.93 | 1.09 | 7.32 | -275 | 5.52 | 1.58 |
| TiRhAs | 1.57 | 6.12 | 1.73 | 9.60 | -278 | 7.43 | 1.80 |
| ZrCoAs | 1.60 | 2.86 | 1.13 | 8.20 | -292 | 7.00 | 2.05 |
| ZrRhAs | 1.85 | 2.12 | 1.27 | 9.24 | -286 | 7.58 | 1.95 |
| HfCoAs | 1.73 | 2.54 | 1.20 | 8.92 | -292 | 7.60 | 2.08 |
| HfRhAs | 2.08 | 1.14 | 1.28 | 6.19 | -179 | 1.97 | 0.47 |
| HfIrAs | 2.50 | 0.29 | 0.77 | 3.94 | -108 | 0.46 | 0.11 |

TABLE S2. Values of physical properties of compounds at the optimal n-doping for maximizing $ZT$ for $\tau = 10^{-14}$s based on HSE band structure.

| | $\kappa_\ell^{\min}$ [W/Km] | p [$10^{20}$/cm$^3$] | $\kappa_e$ [W/Km] | $\sigma$ [$10^4$S/m] | $S$ [$\mu$W/K] | $\mathcal{P}$[mW/K$^2$m] | $ZT$ |
|---|---|---|---|---|---|---|---|
| *stable* | | | | | | | |
| TiNiSn | 1.77 | 2.47 | 1.11 | 7.53 | 263 | 5.22 | 1.45 |
| TiPdSn | 1.53 | 2.28 | 0.97 | 6.24 | 269 | 4.53 | 1.45 |
| TiPtSn | 2.27 | 3.35 | 1.11 | 7.03 | 242 | 4.13 | 0.98 |
| ZrNiSn | 2.22 | 2.23 | 1.11 | 7.63 | 246 | 4.63 | 1.11 |
| ZrPdSn | 1.84 | 1.85 | 1.00 | 6.31 | 245 | 3.80 | 1.07 |
| ZrPtSn | 2.17 | 1.67 | 0.81 | 5.40 | 225 | 2.74 | 0.73 |
| ZrNiPb | 1.32 | 2.05 | 1.16 | 6.63 | 233 | 3.61 | 1.16 |
| ZrPdPb | 1.21 | 1.46 | 0.81 | 4.86 | 245 | 2.91 | 1.16 |
| ZrPtPb | 1.36 | 1.16 | 0.63 | 4.25 | 243 | 2.51 | 1.01 |
| HfNiSn | 1.83 | 2.04 | 1.29 | 7.77 | 233 | 4.23 | 1.09 |
| HfPdSn | 2.03 | 1.61 | 1.05 | 7.01 | 246 | 4.25 | 1.10 |
| HfPtSn | 2.45 | 1.58 | 0.91 | 5.82 | 219 | 2.79 | 0.66 |
| HfNiPb | 1.68 | 2.47 | 1.80 | 9.87 | 201 | 3.99 | 0.92 |
| HfPdPb | 1.54 | 1.65 | 1.04 | 6.33 | 235 | 3.51 | 1.09 |
| HfPtPb | 1.71 | 1.12 | 0.70 | 4.63 | 230 | 2.46 | 0.81 |
| TiCoSb | 2.02 | 3.64 | 1.52 | 8.73 | 280 | 6.82 | 1.54 |
| TiRhSb | 1.85 | 2.60 | 1.20 | 7.02 | 263 | 4.87 | 1.28 |
| TiIrAs | 2.45 | 2.08 | 1.29 | 6.65 | 230 | 3.51 | 0.75 |
| TiIrSb | 2.52 | 2.92 | 1.43 | 7.73 | 238 | 4.39 | 0.89 |
| ZrCoSb | 2.58 | 6.04 | 1.98 | 14.78 | 289 | 12.37 | 2.17 |
| ZrRhSb | 2.08 | 1.59 | 1.13 | 6.36 | 236 | 3.55 | 0.88 |
| ZrCoBi | 1.60 | 2.92 | 1.64 | 8.01 | 265 | 5.61 | 1.39 |
| ZrRhBi | 1.26 | 1.00 | 0.68 | 3.98 | 248 | 2.44 | 1.01 |
| ZrIrAs | 2.34 | 1.26 | 1.31 | 5.97 | 219 | 2.86 | 0.63 |
| ZrIrSb | 2.37 | 1.48 | 1.20 | 6.05 | 224 | 3.03 | 0.68 |
| ZrIrBi | 1.69 | 1.09 | 0.91 | 4.87 | 237 | 2.75 | 0.84 |
| HfCoSb | 2.08 | 2.54 | 1.61 | 8.45 | 269 | 6.14 | 1.33 |
| HfRhSb | 2.23 | 1.42 | 1.09 | 6.95 | 239 | 3.99 | 0.96 |
| HfRhBi | 1.70 | 1.16 | 0.84 | 4.97 | 233 | 2.68 | 0.84 |
| HfIrSb | 3.08 | 1.42 | 1.15 | 6.48 | 206 | 2.75 | 0.52 |
| *unstable* | | | | | | | |
| TiNiPb | 0.91 | 2.32 | 1.13 | 6.54 | 252 | 4.17 | 1.63 |
| TiPdPb | 0.99 | 1.79 | 0.77 | 4.74 | 273 | 3.53 | 1.61 |
| TiPtPb | 1.15 | 2.07 | 0.74 | 4.78 | 274 | 3.60 | 1.53 |
| TiCoBi | 1.12 | 2.11 | 0.89 | 4.86 | 284 | 3.92 | 1.56 |
| TiRhBi | 0.78 | 1.43 | 0.64 | 3.68 | 298 | 3.28 | 1.84 |
| HfCoBi | 2.00 | 1.94 | 1.23 | 6.47 | 242 | 3.80 | 0.94 |
| HfIrBi | 1.97 | 1.42 | 1.34 | 6.70 | 190 | 2.41 | 0.58 |
| TiNiGe | 1.57 | 2.36 | 0.99 | 6.91 | 278 | 5.33 | 1.66 |
| TiPdGe | 1.44 | 2.20 | 0.95 | 6.03 | 275 | 4.56 | 1.53 |
| TiPtGe | 2.14 | 2.80 | 1.05 | 6.47 | 242 | 3.78 | 0.95 |
| ZrNiGe | 1.64 | 1.81 | 0.93 | 6.45 | 265 | 4.52 | 1.40 |
| ZrPdGe | 1.72 | 1.59 | 0.96 | 5.93 | 248 | 3.66 | 1.09 |
| ZrPtGe | 2.21 | 1.41 | 0.80 | 5.14 | 221 | 2.50 | 0.66 |
| HfNiGe | 1.59 | 1.46 | 0.96 | 6.05 | 254 | 3.91 | 1.23 |
| HfPdGe | 1.83 | 1.32 | 0.95 | 6.40 | 253 | 4.09 | 1.17 |
| HfPtGe | 2.54 | 1.34 | 0.89 | 5.56 | 213 | 2.53 | 0.59 |
| TiCoAs | 1.70 | 3.28 | 1.52 | 8.43 | 299 | 7.51 | 1.87 |
| TiRhAs | 1.57 | 1.97 | 1.08 | 6.15 | 267 | 4.39 | 1.32 |
| ZrCoAs | 1.60 | 4.21 | 1.46 | 10.29 | 320 | 10.55 | 2.75 |
| ZrRhAs | 1.85 | 1.27 | 1.10 | 5.93 | 240 | 3.41 | 0.93 |
| HfCoAs | 1.73 | 3.20 | 1.82 | 10.03 | 295 | 8.74 | 1.97 |
| HfRhAs | 2.08 | 1.09 | 1.02 | 6.50 | 240 | 3.74 | 0.96 |
| HfIrAs | 2.50 | 1.31 | 1.36 | 6.70 | 187 | 2.35 | 0.49 |

TABLE S3. Values of physical properties of compounds at the optimal p-doping for maximizing $ZT$ with $\tau = 10^{-14}$s based on HSE band structure.

### B. Results with hybrid functional HSE and $\tau = 0.5 \times 10^{-14}$s

| | $\kappa_\ell^{\min}$ [W/Km] | n [$10^{20}$/cm$^3$] | $\kappa_e$ [W/Km] | $\sigma$ [$10^4$S/m] | $S$ [$\mu$W/K] | $\mathcal{P}$[mW/K$^2$m] | $ZT$ |
|---|---|---|---|---|---|---|---|
| *stable* | | | | | | | |
| TiNiSn | 1.77 | 1.43 | 0.68 | 4.34 | -217 | 2.04 | 0.67 |
| TiPdSn | 1.53 | 2.00 | 0.63 | 3.99 | -225 | 2.03 | 0.75 |
| TiPtSn | 2.27 | 4.94 | 1.09 | 6.40 | -220 | 3.11 | 0.74 |
| ZrNiSn | 2.22 | 1.30 | 0.73 | 4.74 | -209 | 2.08 | 0.56 |
| ZrPdSn | 1.84 | 1.38 | 0.66 | 4.27 | -216 | 1.99 | 0.64 |
| ZrPtSn | 2.17 | 2.34 | 0.74 | 4.72 | -210 | 2.09 | 0.57 |
| ZrNiPb | 1.32 | 1.14 | 0.69 | 4.20 | -217 | 1.97 | 0.78 |
| ZrPdPb | 1.21 | 1.19 | 0.56 | 3.64 | -230 | 1.93 | 0.87 |
| ZrPtPb | 1.36 | 1.89 | 0.58 | 3.75 | -229 | 1.97 | 0.81 |
| HfNiSn | 1.83 | 1.29 | 0.74 | 4.64 | -211 | 2.07 | 0.65 |
| HfPdSn | 2.03 | 1.49 | 0.70 | 4.52 | -213 | 2.06 | 0.60 |
| HfPtSn | 2.45 | 2.44 | 0.77 | 4.95 | -207 | 2.11 | 0.52 |
| HfNiPb | 1.68 | 1.47 | 1.02 | 5.71 | -190 | 2.07 | 0.61 |
| HfPdPb | 1.54 | 1.33 | 0.68 | 4.27 | -219 | 2.04 | 0.73 |
| HfPtPb | 1.71 | 1.97 | 0.66 | 4.21 | -221 | 2.06 | 0.69 |
| TiCoSb | 2.02 | 4.97 | 0.80 | 5.32 | -226 | 2.71 | 0.77 |
| TiRhSb | 1.85 | 9.53 | 0.93 | 6.89 | -244 | 4.09 | 1.18 |
| TiIrAs | 2.45 | 9.20 | 1.98 | 13.47 | -219 | 6.44 | 1.16 |
| TiIrSb | 2.52 | 9.53 | 1.39 | 9.53 | -215 | 4.40 | 0.90 |
| ZrCoSb | 2.58 | 4.67 | 1.00 | 6.60 | -224 | 3.30 | 0.74 |
| ZrRhSb | 2.08 | 4.61 | 0.92 | 5.88 | -233 | 3.18 | 0.85 |
| ZrCoBi | 1.60 | 3.24 | 0.76 | 5.04 | -241 | 2.92 | 0.99 |
| ZrRhBi | 1.26 | 3.24 | 0.70 | 4.78 | -258 | 3.18 | 1.30 |
| ZrIrAs | 2.34 | 43.31 | 12.78 | 68.35 | -74 | 3.77 | 0.20 |
| ZrIrSb | 2.37 | 10.57 | 1.78 | 11.30 | -220 | 5.46 | 1.05 |
| ZrIrBi | 1.69 | 35.44 | 8.65 | 46.57 | -90 | 3.77 | 0.29 |
| HfCoSb | 2.08 | 3.82 | 0.90 | 5.91 | -233 | 3.20 | 0.86 |
| HfRhSb | 2.23 | 4.36 | 0.96 | 6.26 | -230 | 3.33 | 0.83 |
| HfRhBi | 1.70 | 7.03 | 3.05 | 15.71 | -146 | 3.33 | 0.56 |
| HfIrSb | 3.08 | 19.97 | 4.72 | 24.85 | -143 | 5.05 | 0.52 |
| *unstable* | | | | | | | |
| TiNiPb | 0.91 | 1.55 | 0.62 | 3.75 | -225 | 1.90 | 0.99 |
| TiPdPb | 0.99 | 1.97 | 0.49 | 3.27 | -238 | 1.84 | 1.00 |
| TiPtPb | 1.15 | 3.72 | 0.49 | 3.54 | -235 | 1.96 | 0.95 |
| TiCoBi | 1.12 | 3.28 | 0.56 | 3.82 | -247 | 2.34 | 1.11 |
| TiRhBi | 0.78 | 6.21 | 0.51 | 3.66 | -271 | 2.70 | 1.67 |
| HfCoBi | 2.00 | 3.33 | 0.88 | 5.79 | -233 | 3.14 | 0.87 |
| HfIrBi | 1.97 | 0.37 | 0.48 | 2.45 | -93 | 0.21 | 0.07 |
| TiNiGe | 1.57 | 1.92 | 0.63 | 4.19 | -228 | 2.17 | 0.79 |
| TiPdGe | 1.44 | 2.71 | 0.61 | 4.00 | -232 | 2.15 | 0.84 |
| TiPtGe | 2.14 | 7.13 | 1.01 | 6.91 | -234 | 3.77 | 0.96 |
| ZrNiGe | 1.64 | 1.44 | 0.66 | 4.40 | -229 | 2.30 | 0.80 |
| ZrPdGe | 1.72 | 1.74 | 0.67 | 4.48 | -226 | 2.30 | 0.77 |
| ZrPtGe | 2.21 | 3.24 | 0.82 | 5.26 | -217 | 2.48 | 0.65 |
| HfNiGe | 1.59 | 1.38 | 0.66 | 4.38 | -231 | 2.33 | 0.83 |
| HfPdGe | 1.83 | 1.76 | 0.71 | 4.73 | -226 | 2.41 | 0.76 |
| HfPtGe | 2.54 | 3.38 | 0.92 | 5.79 | -213 | 2.63 | 0.61 |
| TiCoAs | 1.70 | 5.83 | 0.81 | 5.43 | -242 | 3.19 | 1.01 |
| TiRhAs | 1.57 | 12.56 | 1.52 | 9.04 | -234 | 4.96 | 1.28 |
| ZrCoAs | 1.60 | 4.21 | 0.84 | 6.04 | -260 | 4.07 | 1.33 |
| ZrRhAs | 1.85 | 3.22 | 0.95 | 6.85 | -254 | 4.41 | 1.26 |
| HfCoAs | 1.73 | 3.75 | 0.89 | 6.54 | -260 | 4.41 | 1.34 |
| HfRhAs | 2.08 | 2.60 | 1.44 | 7.11 | -139 | 1.37 | 0.31 |
| HfIrAs | 2.50 | 0.40 | 0.48 | 2.48 | -98 | 0.24 | 0.06 |

TABLE S4. Values of physical properties of compounds at the optimal n-doping for maximizing $ZT$ for $\tau = 0.5 \times 10^{-14}$s based on HSE band structure.

| | $\kappa_\ell^{\min}$ [W/Km] | p [$10^{20}$/cm$^3$] | $\kappa_e$ [W/Km] | $\sigma$ [$10^4$S/m] | $S$ [$\mu$W/K] | $\mathcal{P}$[mW/K$^2$m] | $ZT$ |
|---|---|---|---|---|---|---|---|
| *stable* | | | | | | | |
| TiNiSn | 1.77 | 3.52 | 0.78 | 5.28 | 236 | 2.93 | 0.92 |
| TiPdSn | 1.53 | 3.42 | 0.73 | 4.64 | 238 | 2.62 | 0.92 |
| TiPtSn | 2.27 | 4.84 | 0.81 | 5.04 | 214 | 2.30 | 0.60 |
| ZrNiSn | 2.22 | 3.07 | 0.76 | 5.22 | 221 | 2.54 | 0.68 |
| ZrPdSn | 1.84 | 2.71 | 0.73 | 4.60 | 216 | 2.14 | 0.67 |
| ZrPtSn | 2.17 | 2.29 | 0.56 | 3.67 | 201 | 1.48 | 0.43 |
| ZrNiPb | 1.32 | 2.58 | 0.70 | 4.16 | 216 | 1.94 | 0.77 |
| ZrPdPb | 1.21 | 2.00 | 0.54 | 3.30 | 221 | 1.61 | 0.74 |
| ZrPtPb | 1.36 | 1.62 | 0.44 | 2.96 | 216 | 1.38 | 0.61 |
| HfNiSn | 1.83 | 2.74 | 0.84 | 5.22 | 211 | 2.33 | 0.70 |
| HfPdSn | 2.03 | 2.26 | 0.73 | 4.89 | 219 | 2.35 | 0.68 |
| HfPtSn | 2.45 | 2.20 | 0.64 | 4.01 | 194 | 1.51 | 0.39 |
| HfNiPb | 1.68 | 2.84 | 0.99 | 5.67 | 191 | 2.08 | 0.62 |
| HfPdPb | 1.54 | 2.15 | 0.66 | 4.16 | 214 | 1.91 | 0.69 |
| HfPtPb | 1.71 | 1.57 | 0.49 | 3.20 | 205 | 1.34 | 0.49 |
| TiCoSb | 2.02 | 5.83 | 1.21 | 6.93 | 244 | 4.11 | 1.02 |
| TiRhSb | 1.85 | 3.99 | 0.92 | 5.37 | 231 | 2.85 | 0.82 |
| TiIrAs | 2.45 | 3.47 | 1.07 | 5.41 | 196 | 2.07 | 0.47 |
| TiIrSb | 2.52 | 4.84 | 1.18 | 6.30 | 203 | 2.60 | 0.56 |
| ZrCoSb | 2.58 | 9.20 | 1.48 | 11.14 | 256 | 7.28 | 1.43 |
| ZrRhSb | 2.08 | 2.49 | 0.89 | 4.91 | 204 | 2.05 | 0.55 |
| ZrCoBi | 1.60 | 6.16 | 1.57 | 8.07 | 219 | 3.88 | 0.98 |
| ZrRhBi | 1.26 | 1.50 | 0.51 | 2.95 | 217 | 1.39 | 0.63 |
| ZrIrAs | 2.34 | 17.15 | 6.20 | 30.14 | 128 | 4.97 | 0.47 |
| ZrIrSb | 2.37 | 2.60 | 1.05 | 5.11 | 188 | 1.81 | 0.42 |
| ZrIrBi | 1.69 | 1.79 | 0.75 | 3.92 | 203 | 1.62 | 0.53 |
| HfCoSb | 2.08 | 4.45 | 1.37 | 7.21 | 231 | 3.83 | 0.89 |
| HfRhSb | 2.23 | 2.07 | 0.80 | 5.02 | 211 | 2.23 | 0.59 |
| HfRhBi | 1.70 | 1.74 | 0.63 | 3.68 | 203 | 1.52 | 0.52 |
| HfIrSb | 3.08 | 2.15 | 0.87 | 4.78 | 178 | 1.52 | 0.31 |
| *unstable* | | | | | | | |
| TiNiPb | 0.91 | 2.88 | 0.66 | 4.02 | 237 | 2.25 | 1.14 |
| TiPdPb | 0.99 | 2.56 | 0.54 | 3.35 | 245 | 2.02 | 1.06 |
| TiPtPb | 1.15 | 3.09 | 0.55 | 3.55 | 242 | 2.08 | 0.98 |
| TiCoBi | 1.12 | 3.42 | 0.72 | 3.92 | 247 | 2.40 | 1.04 |
| TiRhBi | 0.78 | 2.26 | 0.51 | 2.89 | 262 | 1.99 | 1.23 |
| HfCoBi | 2.00 | 3.24 | 1.03 | 5.33 | 207 | 2.28 | 0.60 |
| HfIrBi | 1.97 | 1.89 | 0.85 | 4.37 | 173 | 1.31 | 0.37 |
| TiNiGe | 1.57 | 3.47 | 0.73 | 5.05 | 246 | 3.06 | 1.06 |
| TiPdGe | 1.44 | 3.35 | 0.73 | 4.56 | 242 | 2.66 | 0.98 |
| TiPtGe | 2.14 | 4.10 | 0.77 | 4.70 | 213 | 2.12 | 0.58 |
| ZrNiGe | 1.64 | 2.60 | 0.67 | 4.61 | 235 | 2.55 | 0.88 |
| ZrPdGe | 1.72 | 2.37 | 0.72 | 4.41 | 218 | 2.09 | 0.69 |
| ZrPtGe | 2.21 | 1.96 | 0.55 | 3.52 | 196 | 1.35 | 0.39 |
| HfNiGe | 1.59 | 2.18 | 0.71 | 4.48 | 223 | 2.24 | 0.78 |
| HfPdGe | 1.83 | 1.90 | 0.69 | 4.59 | 224 | 2.29 | 0.73 |
| HfPtGe | 2.54 | 1.88 | 0.63 | 3.85 | 188 | 1.37 | 0.35 |
| TiCoAs | 1.70 | 5.52 | 1.26 | 6.99 | 259 | 4.71 | 1.27 |
| TiRhAs | 1.57 | 3.09 | 0.85 | 4.79 | 233 | 2.60 | 0.86 |
| ZrCoAs | 1.60 | 6.65 | 1.15 | 8.09 | 283 | 6.46 | 1.88 |
| ZrRhAs | 1.85 | 2.04 | 0.87 | 4.66 | 207 | 2.00 | 0.59 |
| HfCoAs | 1.73 | 5.75 | 1.53 | 8.76 | 254 | 5.66 | 1.38 |
| HfRhAs | 2.08 | 1.58 | 0.74 | 4.65 | 212 | 2.08 | 0.59 |
| HfIrAs | 2.50 | 2.07 | 1.03 | 5.08 | 162 | 1.34 | 0.30 |

TABLE S5. Values of physical properties of compounds at the optimal p-doping for maximizing $ZT$ with $\tau = 0.5 \times 10^{-14}$s based on HSE band structure.

### C. Results with GGA functional PBE and $\tau = 10^{-14}$s

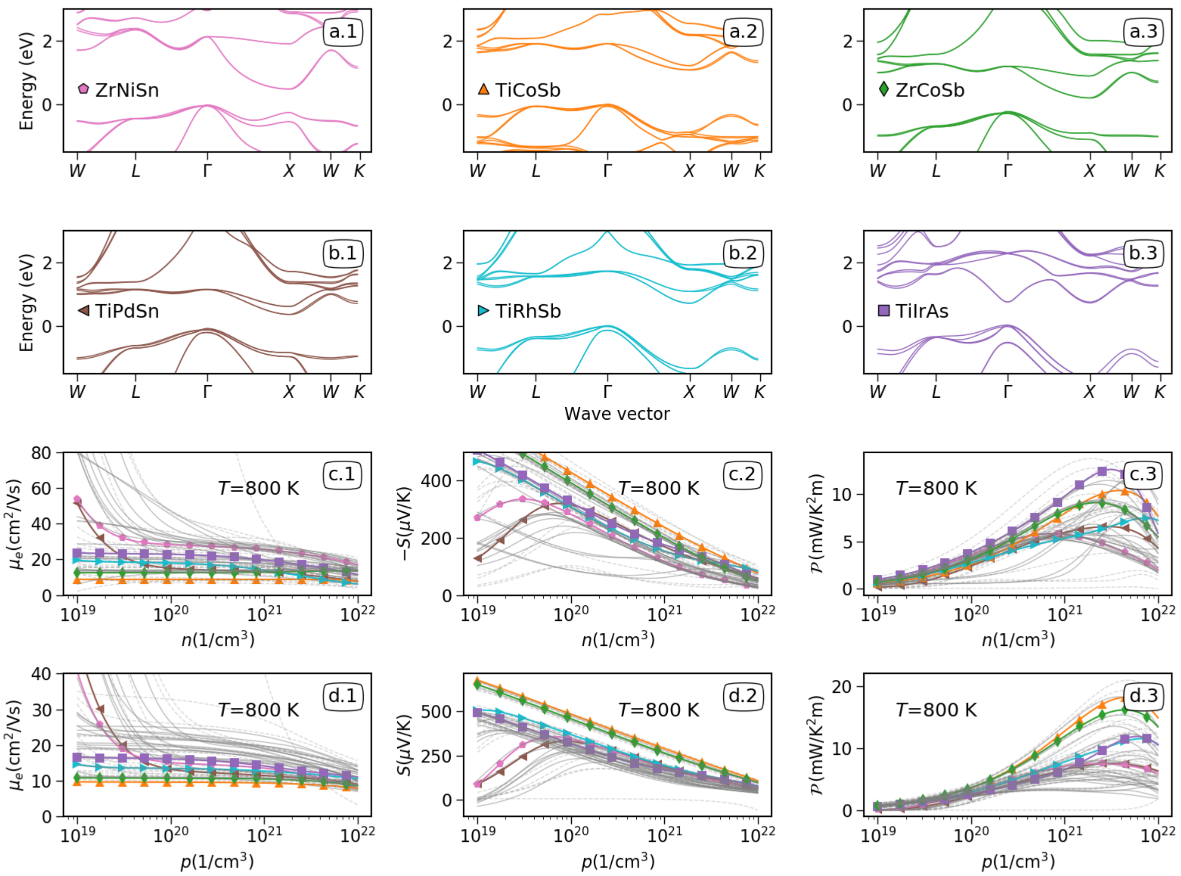


FIG. S3. Band structures and electronic transport properties of group 4 HH alloys. Panels a.1-b.3 show band structures generated at the PBE level (color curves) including spin-orbit coupling for the six selected compositions. Panel c.1 (d.1) displays the electron mobility as a function of n (p) charge carrier concentration, panel c.2 (d.2) shows Pisarenko plots for the n-doped (p-doped) materials, whereas c.3 (d.3) shows corresponding power factors for n-doped (p-doped) compounds. All results are taken at $T = 800$ K. The linestyles in c.1-d.3 are chosen to match the definitions in a.1-b.3, whereas the solid grey curves are results for the other stable alloys and the dashed grey curves for the unstable ones.

| | $\kappa_\ell^{\min}$ [W/Km] | n [$10^{20}$/cm$^3$] | $\kappa_e$ [W/Km] | $\sigma$ [$10^4$S/m] | $S$ [$\mu$W/K] | $\mathcal{P}$[mW/K$^2$m] | $ZT$ |
|---|---|---|---|---|---|---|---|
| *stable* | | | | | | | |
| TiNiSn | 1.77 | 2.67 | 1.62 | 9.13 | -226 | 4.65 | 1.10 |
| TiPdSn | 1.53 | 3.45 | 1.35 | 7.67 | -242 | 4.50 | 1.25 |
| TiPtSn | 2.27 | 5.01 | 1.57 | 9.32 | -246 | 5.66 | 1.18 |
| ZrNiSn | 2.22 | 1.89 | 1.34 | 8.36 | -235 | 4.63 | 1.04 |
| ZrPdSn | 1.84 | 1.51 | 1.19 | 7.20 | -235 | 3.99 | 1.05 |
| ZrPtSn | 2.17 | 2.37 | 1.09 | 6.99 | -245 | 4.19 | 1.03 |
| ZrNiPb | 1.32 | 1.98 | 1.62 | 9.04 | -227 | 4.64 | 1.26 |
| ZrPdPb | 1.21 | 1.80 | 1.42 | 8.01 | -229 | 4.20 | 1.28 |
| ZrPtPb | 1.36 | 1.85 | 0.83 | 5.47 | -265 | 3.85 | 1.41 |
| HfNiSn | 1.83 | 2.15 | 1.87 | 10.31 | -216 | 4.79 | 1.04 |
| HfPdSn | 2.03 | 1.94 | 1.58 | 9.10 | -218 | 4.34 | 0.96 |
| HfPtSn | 2.45 | 2.31 | 1.15 | 7.42 | -238 | 4.22 | 0.94 |
| HfNiPb | 1.68 | 2.84 | 2.80 | 14.27 | -188 | 5.04 | 0.90 |
| HfPdPb | 1.54 | 2.28 | 2.13 | 11.19 | -202 | 4.58 | 1.00 |
| HfPtPb | 1.71 | 1.85 | 0.98 | 6.20 | -256 | 4.07 | 1.21 |
| TiCoSb | 2.02 | 6.47 | 1.37 | 9.12 | -273 | 6.78 | 1.60 |
| TiRhSb | 1.85 | 2.15 | 1.02 | 5.97 | -249 | 3.70 | 1.03 |
| TiIrAs | 2.45 | 2.71 | 1.86 | 9.56 | -251 | 6.01 | 1.11 |
| TiIrSb | 2.52 | 2.51 | 1.38 | 7.64 | -236 | 4.25 | 0.87 |
| ZrCoSb | 2.58 | 4.84 | 1.46 | 9.85 | -259 | 6.63 | 1.31 |
| ZrRhSb | 2.08 | 4.61 | 1.47 | 9.46 | -276 | 7.21 | 1.62 |
| ZrCoBi | 1.60 | 3.52 | 1.09 | 7.56 | -283 | 6.07 | 1.81 |
| ZrRhBi | 1.26 | 3.17 | 1.01 | 7.04 | -304 | 6.49 | 2.29 |
| ZrIrAs | 2.34 | 38.78 | 23.11 | 123.68 | -79 | 7.69 | 0.24 |
| ZrIrSb | 2.37 | 1.52 | 1.28 | 6.37 | -236 | 3.54 | 0.77 |
| ZrIrBi | 1.69 | 43.92 | 16.86 | 94.40 | -88 | 7.32 | 0.32 |
| HfCoSb | 2.08 | 3.88 | 1.30 | 8.70 | -270 | 6.36 | 1.50 |
| HfRhSb | 2.23 | 3.90 | 1.38 | 8.87 | -266 | 6.27 | 1.39 |
| HfRhBi | 1.70 | 10.42 | 8.36 | 40.86 | -119 | 5.74 | 0.46 |
| HfIrSb | 3.08 | 34.48 | 14.18 | 76.11 | -119 | 10.81 | 0.50 |
| *unstable* | | | | | | | |
| TiNiPb | 0.91 | 4.10 | 2.02 | 10.95 | -207 | 4.70 | 1.28 |
| TiPdPb | 0.99 | 4.36 | 1.53 | 8.57 | -225 | 4.33 | 1.38 |
| TiPtPb | 1.15 | 6.93 | 0.89 | 7.37 | -289 | 6.14 | 2.41 |
| TiCoBi | 1.12 | 4.71 | 0.84 | 6.08 | -293 | 5.21 | 2.13 |
| TiRhBi | 0.78 | 2.92 | 0.78 | 4.36 | -305 | 4.07 | 2.09 |
| HfCoBi | 2.00 | 3.62 | 1.30 | 8.97 | -276 | 6.83 | 1.66 |
| HfIrBi | 1.97 | 1.34 | 1.95 | 9.40 | -91 | 0.77 | 0.16 |
| TiNiGe | 1.57 | 2.49 | 1.02 | 6.75 | -260 | 4.58 | 1.41 |
| TiPdGe | 1.44 | 3.42 | 1.14 | 7.02 | -279 | 5.48 | 1.70 |
| TiPtGe | 2.14 | 2.04 | 1.11 | 6.35 | -243 | 3.74 | 0.92 |
| ZrNiGe | 1.64 | 1.69 | 1.02 | 6.83 | -264 | 4.78 | 1.43 |
| ZrPdGe | 1.72 | 1.75 | 1.00 | 6.69 | -259 | 4.48 | 1.32 |
| ZrPtGe | 2.21 | 3.20 | 1.27 | 7.85 | -256 | 5.13 | 1.18 |
| HfNiGe | 1.59 | 1.67 | 1.12 | 7.20 | -261 | 4.90 | 1.45 |
| HfPdGe | 1.83 | 1.78 | 1.12 | 7.31 | -255 | 4.76 | 1.29 |
| HfPtGe | 2.54 | 3.22 | 1.42 | 8.68 | -251 | 5.46 | 1.10 |
| TiCoAs | 1.70 | 6.84 | 1.33 | 9.37 | -297 | 8.26 | 2.18 |
| TiRhAs | 1.57 | 1.66 | 0.97 | 5.44 | -258 | 3.61 | 1.14 |
| ZrCoAs | 1.60 | 4.18 | 1.18 | 8.58 | -298 | 7.61 | 2.19 |
| ZrRhAs | 1.85 | 2.82 | 1.38 | 10.10 | -296 | 8.84 | 2.19 |
| HfCoAs | 1.73 | 3.69 | 1.25 | 9.48 | -297 | 8.38 | 2.25 |
| HfRhAs | 2.08 | 0.72 | 0.83 | 4.19 | -167 | 1.17 | 0.32 |
| HfIrAs | 2.50 | 1.54 | 2.12 | 10.34 | -95 | 0.94 | 0.16 |

TABLE S6. Values of physical properties of compounds at the optimal n-doping for maximizing $ZT$ for $\tau = 10^{-14}$s based on PBE band structure.

### D. Results with GGA functional PBE and $\tau = 0.5 \times 10^{-14}$s

| | $\kappa_\ell^{\min}$ [W/Km] | n [$10^{20}$/cm$^3$] | $\kappa_e$ [W/Km] | $\sigma$ [$10^4$S/m] | $S$ [$\mu$W/K] | $\mathcal{P}$[mW/K$^2$m] | $ZT$ |
|---|---|---|---|---|---|---|---|
| *stable* | | | | | | | |
| TiNiSn | 1.77 | 3.35 | 0.95 | 5.63 | -210 | 2.49 | 0.73 |
| TiPdSn | 1.53 | 4.58 | 0.85 | 5.02 | -222 | 2.47 | 0.83 |
| TiPtSn | 2.27 | 8.89 | 1.27 | 7.68 | -210 | 3.40 | 0.77 |
| ZrNiSn | 2.22 | 2.53 | 0.87 | 5.54 | -213 | 2.52 | 0.65 |
| ZrPdSn | 1.84 | 2.04 | 0.77 | 4.78 | -213 | 2.18 | 0.67 |
| ZrPtSn | 2.17 | 3.42 | 0.79 | 5.02 | -216 | 2.35 | 0.63 |
| ZrNiPb | 1.32 | 2.37 | 0.91 | 5.36 | -214 | 2.46 | 0.88 |
| ZrPdPb | 1.21 | 2.17 | 0.81 | 4.78 | -216 | 2.23 | 0.88 |
| ZrPtPb | 1.36 | 2.73 | 0.61 | 4.00 | -234 | 2.20 | 0.89 |
| HfNiSn | 1.83 | 2.60 | 1.06 | 6.16 | -203 | 2.53 | 0.70 |
| HfPdSn | 2.03 | 2.41 | 0.94 | 5.59 | -203 | 2.31 | 0.62 |
| HfPtSn | 2.45 | 3.31 | 0.83 | 5.29 | -210 | 2.34 | 0.57 |
| HfNiPb | 1.68 | 3.17 | 1.48 | 7.89 | -182 | 2.60 | 0.66 |
| HfPdPb | 1.54 | 2.61 | 1.16 | 6.37 | -194 | 2.39 | 0.71 |
| HfPtPb | 1.71 | 2.73 | 0.72 | 4.54 | -226 | 2.32 | 0.76 |
| TiCoSb | 2.02 | 9.79 | 1.04 | 6.91 | -239 | 3.96 | 1.03 |
| TiRhSb | 1.85 | 3.31 | 0.77 | 4.42 | -218 | 2.11 | 0.64 |
| TiIrAs | 2.45 | 5.59 | 1.80 | 9.39 | -206 | 3.97 | 0.75 |
| TiIrSb | 2.52 | 4.18 | 1.13 | 6.13 | -202 | 2.49 | 0.55 |
| ZrCoSb | 2.58 | 6.98 | 1.07 | 7.15 | -229 | 3.75 | 0.82 |
| ZrRhSb | 2.08 | 6.93 | 1.12 | 7.19 | -243 | 4.23 | 1.06 |
| ZrCoBi | 1.60 | 5.22 | 0.82 | 5.63 | -251 | 3.53 | 1.17 |
| ZrRhBi | 1.26 | 4.87 | 0.78 | 5.42 | -268 | 3.89 | 1.53 |
| ZrIrAs | 2.34 | 39.59 | 11.64 | 62.80 | -79 | 3.87 | 0.22 |
| ZrIrSb | 2.37 | 35.44 | 6.13 | 33.95 | -126 | 5.42 | 0.51 |
| ZrIrBi | 1.69 | 44.84 | 8.47 | 47.81 | -88 | 3.68 | 0.29 |
| HfCoSb | 2.08 | 5.71 | 0.97 | 6.44 | -239 | 3.66 | 0.96 |
| HfRhSb | 2.23 | 5.83 | 1.04 | 6.64 | -234 | 3.62 | 0.88 |
| HfRhBi | 1.70 | 11.64 | 4.46 | 22.43 | -116 | 3.02 | 0.39 |
| HfIrSb | 3.08 | 37.46 | 7.35 | 40.59 | -117 | 5.56 | 0.43 |
| *unstable* | | | | | | | |
| TiNiPb | 0.91 | 4.48 | 1.06 | 5.94 | -202 | 2.42 | 0.98 |
| TiPdPb | 0.99 | 5.08 | 0.84 | 4.93 | -215 | 2.27 | 1.00 |
| TiPtPb | 1.15 | 10.42 | 0.64 | 5.40 | -257 | 3.56 | 1.59 |
| TiCoBi | 1.12 | 7.13 | 0.63 | 4.58 | -259 | 3.07 | 1.40 |
| TiRhBi | 0.78 | 5.04 | 0.63 | 3.59 | -267 | 2.55 | 1.45 |
| HfCoBi | 2.00 | 5.33 | 0.97 | 6.63 | -244 | 3.94 | 1.06 |
| HfIrBi | 1.97 | 1.45 | 1.02 | 5.01 | -88 | 0.39 | 0.11 |
| TiNiGe | 1.57 | 3.52 | 0.71 | 4.74 | -233 | 2.57 | 0.90 |
| TiPdGe | 1.44 | 5.26 | 0.86 | 5.35 | -246 | 3.24 | 1.13 |
| TiPtGe | 2.14 | 3.17 | 0.85 | 4.74 | -212 | 2.13 | 0.57 |
| ZrNiGe | 1.64 | 2.42 | 0.73 | 4.88 | -235 | 2.70 | 0.91 |
| ZrPdGe | 1.72 | 2.51 | 0.72 | 4.77 | -230 | 2.52 | 0.83 |
| ZrPtGe | 2.21 | 4.74 | 0.95 | 5.82 | -225 | 2.94 | 0.74 |
| HfNiGe | 1.59 | 2.32 | 0.76 | 5.00 | -235 | 2.75 | 0.93 |
| HfPdGe | 1.83 | 2.51 | 0.79 | 5.15 | -228 | 2.67 | 0.81 |
| HfPtGe | 2.54 | 4.80 | 1.07 | 6.49 | -219 | 3.12 | 0.69 |
| TiCoAs | 1.70 | 10.35 | 1.02 | 7.16 | -262 | 4.91 | 1.45 |
| TiRhAs | 1.57 | 2.61 | 0.75 | 4.18 | -225 | 2.11 | 0.73 |
| ZrCoAs | 1.60 | 6.21 | 0.88 | 6.39 | -264 | 4.46 | 1.43 |
| ZrRhAs | 1.85 | 4.33 | 1.04 | 7.59 | -262 | 5.20 | 1.44 |
| HfCoAs | 1.73 | 5.44 | 0.93 | 6.99 | -264 | 4.89 | 1.47 |
| HfRhAs | 2.08 | 2.69 | 1.46 | 7.08 | -112 | 0.88 | 0.20 |
| HfIrAs | 2.50 | 1.62 | 1.09 | 5.41 | -93 | 0.47 | 0.11 |

TABLE S7. Values of physical properties of compounds at the optimal n-doping for maximizing $ZT$ for $\tau = 0.5 \times 10^{-14}$s based on PBE band structure.

| | $\kappa_\ell^{\min}$ [W/Km] | p [$10^{20}$/cm$^3$] | $\kappa_e$ [W/Km] | $\sigma$ [$10^4$S/m] | $S$ [$\mu$W/K] | $\mathcal{P}$[mW/K$^2$m] | $ZT$ |
|---|---|---|---|---|---|---|---|
| *stable* | | | | | | | |
| TiNiSn | 1.77 | 6.29 | 1.03 | 6.36 | 227 | 3.27 | 0.94 |
| TiPdSn | 1.53 | 5.63 | 0.92 | 5.36 | 228 | 2.78 | 0.91 |
| TiPtSn | 2.27 | 5.67 | 0.76 | 4.68 | 210 | 2.06 | 0.54 |
| ZrNiSn | 2.22 | 5.44 | 0.95 | 6.17 | 225 | 3.11 | 0.79 |
| ZrPdSn | 1.84 | 3.99 | 0.84 | 5.15 | 216 | 2.40 | 0.72 |
| ZrPtSn | 2.17 | 2.92 | 0.57 | 3.72 | 202 | 1.52 | 0.44 |
| ZrNiPb | 1.32 | 4.55 | 0.98 | 5.60 | 216 | 2.61 | 0.91 |
| ZrPdPb | 1.21 | 3.54 | 0.85 | 4.55 | 207 | 1.96 | 0.76 |
| ZrPtPb | 1.36 | 2.07 | 0.45 | 3.05 | 217 | 1.44 | 0.63 |
| HfNiSn | 1.83 | 4.64 | 1.12 | 6.53 | 203 | 2.70 | 0.73 |
| HfPdSn | 2.03 | 3.35 | 0.97 | 5.97 | 210 | 2.63 | 0.70 |
| HfPtSn | 2.45 | 2.74 | 0.66 | 4.15 | 196 | 1.59 | 0.41 |
| HfNiPb | 1.68 | 4.84 | 1.42 | 7.55 | 177 | 2.36 | 0.61 |
| HfPdPb | 1.54 | 3.72 | 1.11 | 6.11 | 189 | 2.18 | 0.66 |
| HfPtPb | 1.71 | 1.96 | 0.52 | 3.33 | 205 | 1.40 | 0.50 |
| TiCoSb | 2.02 | 13.46 | 1.18 | 10.08 | 266 | 7.11 | 1.78 |
| TiRhSb | 1.85 | 5.56 | 1.05 | 5.82 | 235 | 3.21 | 0.89 |
| TiIrAs | 2.45 | 6.21 | 1.56 | 7.38 | 192 | 2.73 | 0.54 |
| TiIrSb | 2.52 | 6.74 | 1.31 | 6.86 | 204 | 2.85 | 0.60 |
| ZrCoSb | 2.58 | 12.05 | 1.35 | 10.14 | 250 | 6.34 | 1.29 |
| ZrRhSb | 2.08 | 4.30 | 1.23 | 6.28 | 220 | 3.03 | 0.73 |
| ZrCoBi | 1.60 | 9.20 | 1.07 | 7.89 | 265 | 5.55 | 1.67 |
| ZrRhBi | 1.26 | 2.61 | 0.71 | 3.78 | 230 | 2.00 | 0.81 |
| ZrIrAs | 2.34 | 9.59 | 2.92 | 14.83 | 183 | 4.95 | 0.75 |
| ZrIrSb | 2.37 | 9.33 | 2.58 | 12.92 | 177 | 4.06 | 0.65 |
| ZrIrBi | 1.69 | 3.80 | 1.21 | 6.29 | 204 | 2.62 | 0.72 |
| HfCoSb | 2.08 | 11.89 | 1.16 | 10.28 | 265 | 7.24 | 1.78 |
| HfRhSb | 2.23 | 2.82 | 0.89 | 5.50 | 222 | 2.70 | 0.69 |
| HfRhBi | 1.70 | 2.60 | 0.77 | 4.39 | 214 | 2.01 | 0.65 |
| HfIrSb | 3.08 | 3.99 | 1.36 | 6.83 | 176 | 2.11 | 0.38 |
| *unstable* | | | | | | | |
| TiNiPb | 0.91 | 5.87 | 1.13 | 5.97 | 206 | 2.53 | 0.99 |
| TiPdPb | 0.99 | 5.33 | 0.94 | 4.94 | 215 | 2.28 | 0.95 |
| TiPtPb | 1.15 | 3.69 | 0.54 | 3.40 | 234 | 1.86 | 0.88 |
| TiCoBi | 1.12 | 7.69 | 0.84 | 6.00 | 279 | 4.66 | 1.90 |
| TiRhBi | 0.78 | 3.11 | 0.57 | 3.15 | 267 | 2.24 | 1.33 |
| HfCoBi | 2.00 | 8.71 | 1.11 | 8.52 | 256 | 5.59 | 1.43 |
| HfIrBi | 1.97 | 8.18 | 2.66 | 12.99 | 140 | 2.55 | 0.44 |
| TiNiGe | 1.57 | 5.40 | 0.84 | 5.56 | 251 | 3.50 | 1.16 |
| TiPdGe | 1.44 | 4.61 | 0.79 | 4.76 | 241 | 2.77 | 0.99 |
| TiPtGe | 2.14 | 4.84 | 0.74 | 4.44 | 210 | 1.96 | 0.54 |
| ZrNiGe | 1.64 | 5.01 | 0.91 | 5.68 | 252 | 3.59 | 1.13 |
| ZrPdGe | 1.72 | 3.38 | 0.78 | 4.79 | 224 | 2.41 | 0.77 |
| ZrPtGe | 2.21 | 2.56 | 0.58 | 3.64 | 198 | 1.43 | 0.41 |
| HfNiGe | 1.59 | 3.40 | 0.82 | 5.14 | 231 | 2.74 | 0.91 |
| HfPdGe | 1.83 | 2.51 | 0.77 | 5.09 | 227 | 2.61 | 0.80 |
| HfPtGe | 2.54 | 2.44 | 0.68 | 4.11 | 190 | 1.48 | 0.37 |
| TiCoAs | 1.70 | 11.97 | 1.10 | 9.57 | 283 | 7.68 | 2.19 |
| TiRhAs | 1.57 | 4.24 | 0.97 | 5.23 | 243 | 3.08 | 0.97 |
| ZrCoAs | 1.60 | 7.90 | 1.03 | 7.19 | 272 | 5.32 | 1.61 |
| ZrRhAs | 1.85 | 3.75 | 1.32 | 6.38 | 226 | 3.25 | 0.82 |
| HfCoAs | 1.73 | 10.00 | 1.17 | 9.00 | 276 | 6.86 | 1.89 |
| HfRhAs | 2.08 | 2.04 | 0.85 | 5.20 | 223 | 2.58 | 0.70 |
| HfIrAs | 2.50 | 20.10 | 5.95 | 29.15 | 131 | 5.01 | 0.47 |

TABLE S8. Values of physical properties of compounds at the optimal p-doping for maximizing $ZT$ for $\tau = 0.5 \times 10^{-14}$s based on PBE band structure.

### E. Results with HSE functional and $\tau = 10^{-14}$s at $T = 300$K

Results for electronic properties and $ZT$ at 300 K is provided here. Figure S1 provides thermal conductivity at 300 K.

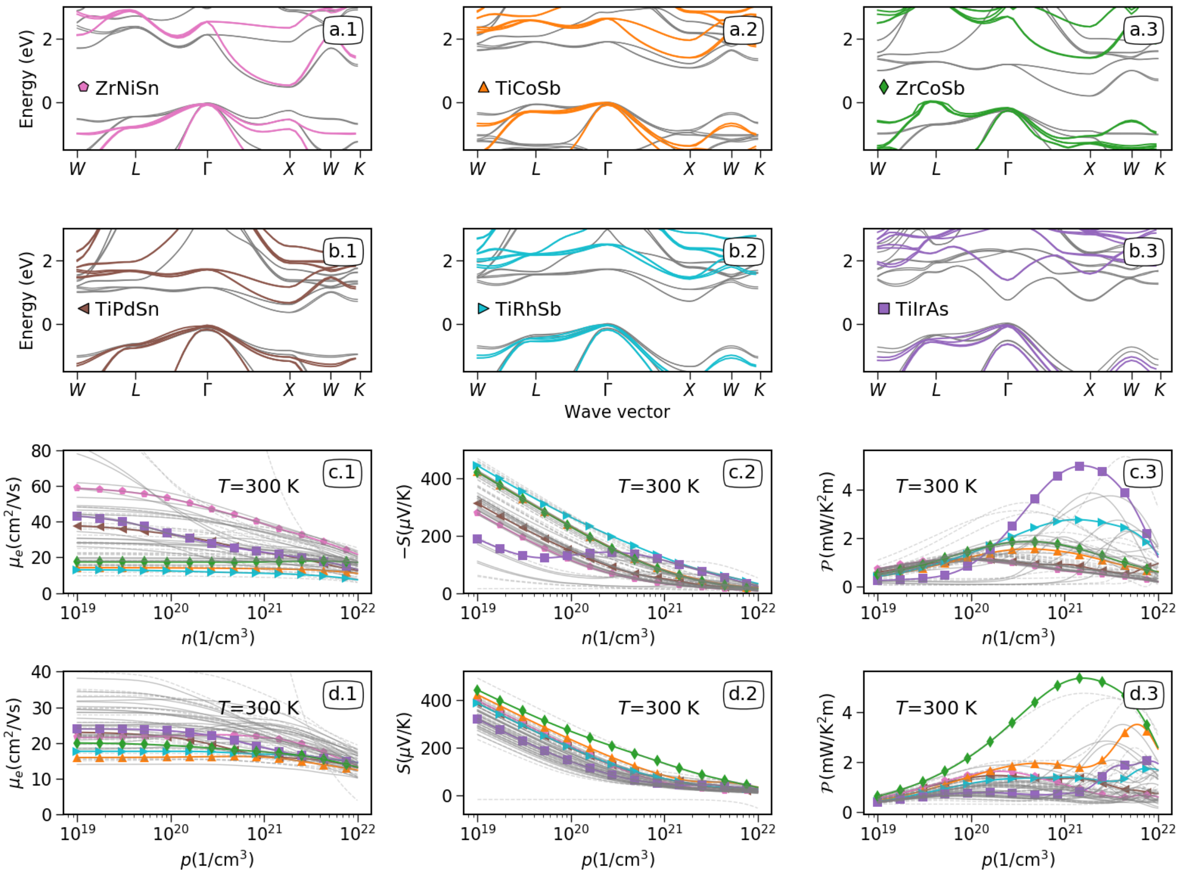


FIG. S4. Band structures and electronic transport properties of group 4 HH alloys. Panels a.1-b.3 show band structures generated at the HSE level (color curves) including spin-orbit coupling for the six selected compositions. Panel c.1 (d.1) displays the electron mobility as a function of n (p) charge carrier concentration, panel c.2 (d.2) shows Pisarenko plots for the n-doped (p-doped) materials, whereas c.3 (d.3) shows corresponding power factors for n-doped (p-doped) compounds. All results are taken at $T = 300$ K. The linestyles in c.1-d.3 are chosen to match the definitions in a.1-b.3, whereas the solid grey curves are results for the other stable alloys and the dashed grey curves for the unstable ones.

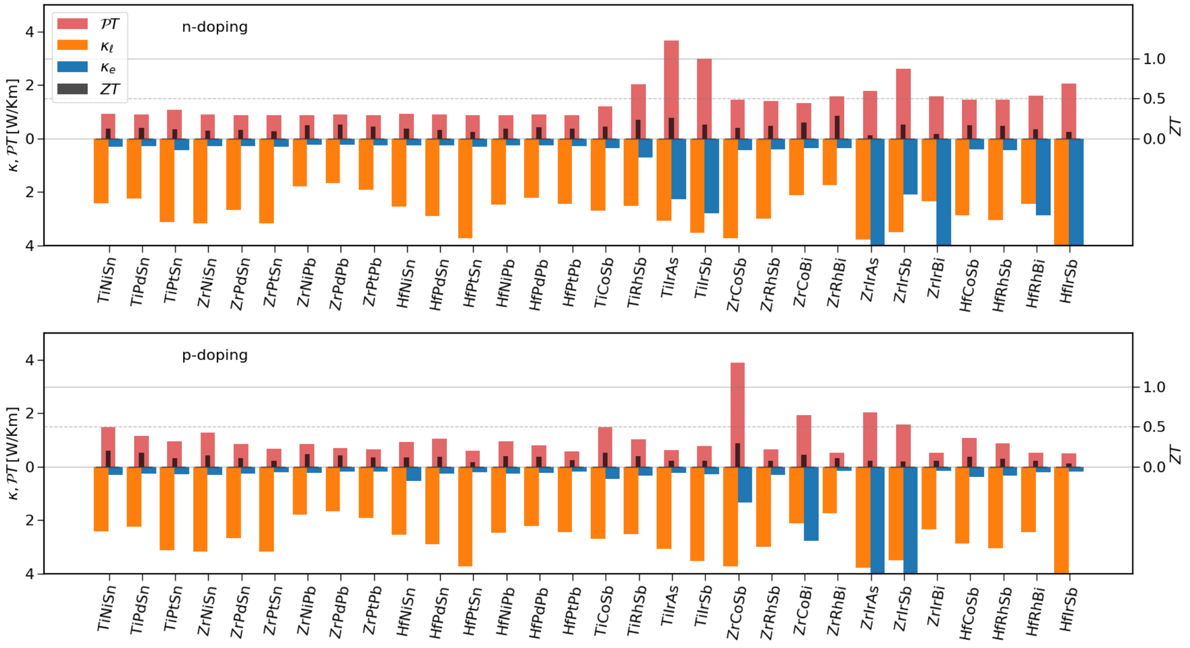


FIG. S5. The predicted optimal $ZT$ values (black, thin bars) of the 30 stable HH alloys at $T = 300$ K, based on the calculations for 300 K. The corresponding power factor times temperature $\mathcal{P}T$ is shown as red bars, and the phonon (electronic) part of the thermal conductivity $\kappa_\ell$ ($\kappa_\mathrm{e}$) is shown as yellow (blue) bars. Results for optimal n-doping (p-doping) are shown in the upper (lower) panel.
